# Supplementary material for: Physics with CEBAF at 12 GeV and Future Opportunities
Source: arXiv:2112.00060 source file (2022-08-10)
Supplement: Supplementary file 1 [file AppendixC_old.tex]

\section{ Appendix C: CEBAF Energy Upgrade ( S.A. Bogacz, L.  Harwood, G. Krafft)}
%
\subsection{Modern Fixed Field Alternating Gradient (FFA) Technology }
 The Cornell-BNL ERL Test Accelerator (CBETA) aims at demonstrating eight-pass beam recirculation with energy recovery (four accelerating beam passes and four decelerating beam passes) through a complete TESLA-style SRF cryomodule. CBETA facility, if successful, would demonstrate simultaneous transport of multiple  beams with energies spanning a factor of 4, through a single beamline configured with fixed-field permanent magnets.
%

\subsection{Energy 'Doubling' Scheme} 
Encouraged by recent success of CBETA, a proposal was formulated to increase CEBAF energy from the present \SI{12}{~GeV} to \SI{20-24}{~GeV} by replacing the highest-energy arcs, ARC 9 and Arc A, with a pair of Fixed Field Alternating-Gradient (FFA) arcs to recirculate the beam for 6-7 additional passes. Above scheme would nearly double the energy using the existing CEBAF SRF cavity system. The new pair of arcs configured with FFA lattice would support simultaneous transport of 6-7 passes with energies spanning a factor of two. 
The design schematic is shown in Fig.~\ref{fig:FFA_CEBAF} In the accelerator passes 1-4 would be accomplished through the current \SI{12}{~GeV} CEBAF. Passes 5-10 (six passes) would be facilitated by constructing two 'CBETA-like' beam-lines indicated schematically in the figure below. 
Staying within CEBAF footprint, while transporting high energy beams calls for increase of the bend radius at the arc dipoles, to suppress adverse effects of the synchrotron radiation on beam quality. The bender packing efficiency is about  \SI{87.6~}\si{\%}, leading to a bending magnetic field requirement of \SI{9 ± 3}{~kG}, and a field gradient requirement of about \SI{3}{~kG/cm} to allow a \SI{1}{~cm} beam aperture. One of the immediate accelerator design tasks is to develop a proof-of-principle FFA arc cell.  Here, we examine a possibility of using combined function magnets to configure a cascade, six- or seven-way beam split switchyard. 
Finally, a novel multi-pass linac optics based on triplet focusing lattice configured with permanent magnets is being explored.
%
\begin{figure}[tbh]
  \centering
  \includegraphics[width=0.8\textwidth]{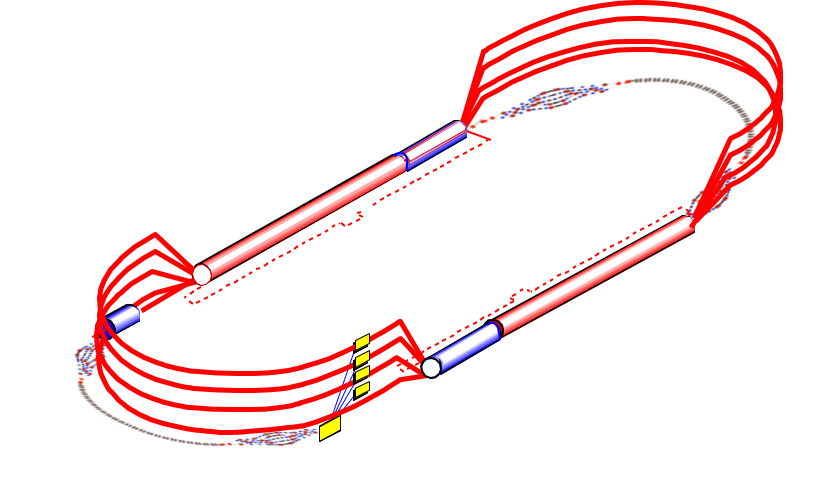}
  \caption{Schematic layout of FFA CEBAF.}
  \label{fig:FFA_CEBAF}
\end{figure}
%
\subsection{Synchrotron Radiation Effects on Beam Quality}
Arc optics was designed to ease individual adjustment of momentum compaction and the horizontal emittance  dispersion, $H$, in each arc.
Tab.~\ref{tab:SREmittance} lists arc-by-arc dilution of the transverse, $\Delta \epsilon$, and longitudinal, $\Delta \sigma_{\frac{\Delta E}{E}}$, emittance due to quantum excitations calculated using analytic formulas:  
%
\begin{equation}
  \Delta E = \frac{2 \pi}{3} r_0 ~mc^2~ \frac{\gamma^4}{\rho}\,
  \label{eq:Emit_dil_1}
\end{equation}
%
\begin{equation}
  \Delta \epsilon_N = \frac{2 \pi}{3} C_q r_0 <H> \frac{\gamma^6}{\rho^2}\,,
  \label{eq:Emit_dil_2}
\end{equation}
%
\begin{equation}
  \frac{\Delta \epsilon_E^2}{E^2} = \frac{2 \pi}{3} C_q r_0~ \frac{\gamma^5}{\rho^2}\,,
  \label{eq:Emit_dil_3}
\end{equation}

Here, $\Delta \epsilon^2_E$ is an increment of energy square variance, $r_0$ is the classical electron radius, $\gamma$ is the Lorentz boost and C_q = \frac{55}{32 \sqrt{3}} \frac{\hbar}{m c} \approx 3.832 \cdot 10^{-13}\,\text{m}$ for electrons (or positrons).
The horizontal emittance dispersion in Eq.~\ref{eq:Emit_dil_2},  is given by the following formula: $H = (1+\alpha^2)/\beta \cdot D^2 + 2 \alpha \ D D' + \beta \cdot D'^2$ where $D, D'$ are the bending plane dispersion and its derivative, with averaging over bends defined as: $<...>~=~\frac{1}{\pi}\int_\text{bends}...~\text{d}\theta$.




\begin{table}[!ht]
  \centering
  \small
  \begin{tabular}{lccccc} 
  \hline
  %\toprule
  Beamline & Beam Energy & $\rho$ & $\Delta E$  & $\Delta \epsilon^x_N$ & $\Delta \sigma_{\frac{\Delta E}{E}}$  \\
    & [\si{GeV}] & [\si{m}] & [\si{MeV}]&  [\si{mm~mrad}] &  [\si{\%}]\\
  \hline\hline
  %\midrule
  Arc 1 & 1.2 & 5.1 & 0.02 & 0.003 & 0.0003\\
  ... & ... & ... & ... & ... & ...\\
  Arc 8 & 8.8 & 30.6 & 9 & 12 & 0.022\\
  FFA 9 & 9.91 & 70.6 & 6 & 13 & 0.026\\
  ... & ... & ... & ... & ... & ...\\
  FFA 19 & 20.44 & 70.6 & 109 & 37 & 0.15\\
  FFA 20 & 21.42 & 70.6 & 132 & 47 & 0.17\\
  FFA 21 & 22.38 & 70.6 & 157 & 60 & 0.020\\
  FFA 22 & 23.31 & 70.6 & 185 & 76 & 0.023\\
  \hline
  %\bottomrule
  \end{tabular}
  \caption{Energy loss and cummulative emittance dilution (horizontal and longitudinal) due to synchroton radiation at the end of selected  \SI{180}{-degree} arcs (not including Spreaders, Recombiners and Doglegs). Here, $\Delta \sigma_{\frac{\Delta E}{E}} = \sqrt{\tfrac{\Delta \epsilon_E^2}{E^2}}$}.
  \label{tab:SREmittance}
\end{table}
%
The beam parameters of the final design are \SI{23}{~GeV} beam energy, a delivered normalized beam emittance of  is \SI{76}{~mm~mrad}, and a relative energy spread of $2.3 \cdot 10^{-3}$. Interestingly, \SI{976}{~MeV} beam energy per electron is lost to synchrotron radiation in traversing the accelerator.
